# Supplementary material for: Learning to Generate Cost-to-Go Functions for Efficient Motion Planning
Source: arXiv:2010.14597 source file (2020-10-27)
Supplement: Supplementary file 1 [file supplementary.tex]

\newpage
\section{Supplementary}

\section{Introduction}
% There is a theory which states that if ever anyone discovers exactly what the Universe is for and why it is here, it will instantly disappear and be replaced by something even more bizarre and inexplicable.
% \jinwook{draw a main figure, write more overview of project}
\begin{figure}[h!]
\centering
\includegraphics[width=0.9\textwidth]{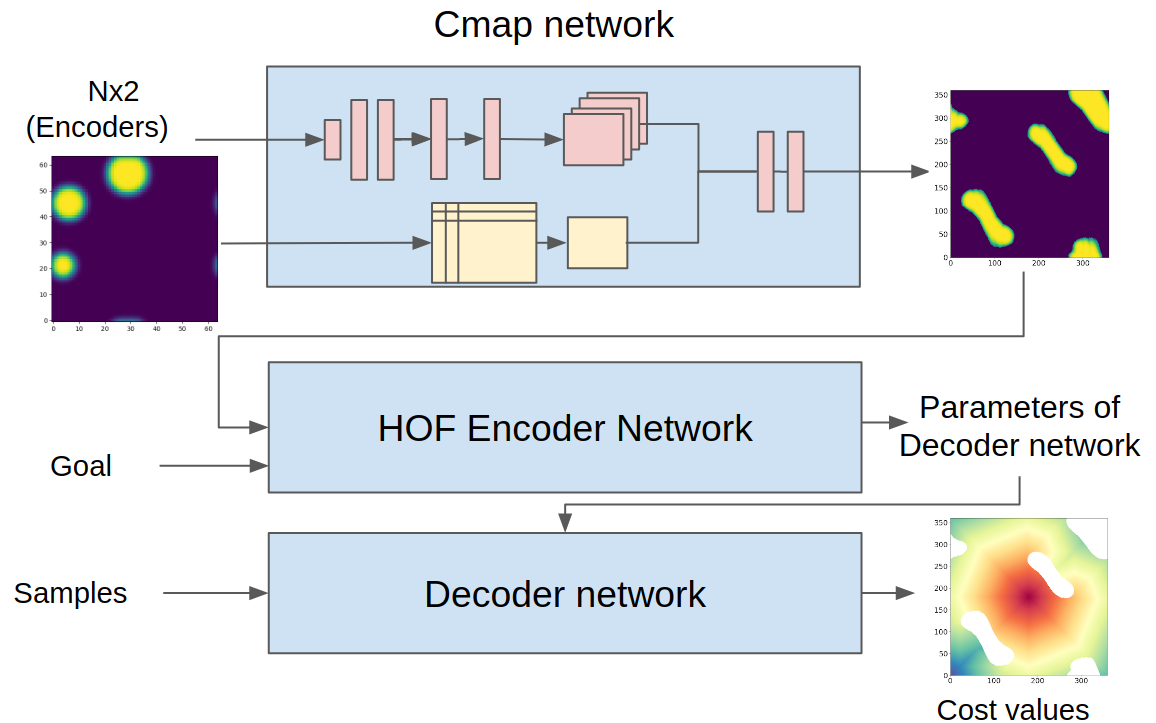}
\caption{The overall network}
\label{fig:universe}
\end{figure}

\begin{itemize}
    \item Motion planning algorithm requires to generate collision-free trajectories rapidly. 
    \item There are search-based planning approaches such as A* and D* to compute optimal paths. However these search-based planning algorithms require discretization of space and they are computationally intractable in high-dimensional space.
    \item Sampling based planning approaches such as Probabilistic RoadMap (PRM) and Randomly exploring Random Trees (RRT) are popular due to their simplicity and flexibility in the high-dimensional space, but they have disadvantages that their performance depends on sampling and local steering algorithms. Although there are many variation of sampling based planning approaches to overcome these limitations, it is very hard to overcome a critical disadvantage that the performance is dramatically degraded in complicated configuration spaces.
    \item To address problems of traditional planning approaches, we suggest a learning approach with deep neural networks. Given workspace information and a goal configuration, the neural network estimates the cost values in the configuration space. Since the suggested deep neural network can estimate cost values without heavy computation, it help a planner to generate a trajectory quickly. In addition, since the network estimates cost values in C-space, it is unnecessary to find mapping between workspace and C-space using inverse and forward kinematics.
    % \item Compared to other planning neural networks, .....
\end{itemize}

Contribution of this paper
\begin{itemize}
     \item This paper suggests a novel network for cost estimation of configuration space with three layers; 1) cmap network to generate a probability of collision in C-space, 2) High Order Functions (HOF) network for learning of parameters of secondary network, and 3)  secondary network to predict cost-to-go of sample configurations considering collisions.
     \item The suggested network generates cost values given samples with workspace information by end-to-end approach from workspace to cost values. 
     \item The Cmap network has an advantage to estimate collision probability of a lot of configuration samples instantly; thus it generates collision map of configuration space instantly.
     \item HOF network is a neural network encodes the information of camp into the weights and biases of the secondary decoder network and the decoder network predicts cost values of sample configurations.
    \item Since the decoder network has small number of parameters compared to other previous planning networks, it is very efficient for fast planning. In addition, when the environment is changed, the encoder network quickly update the weights and biases of decoder network, it is also applicable to changing environments without heavy computation.
    \item The paper proposes a fast trajectory generation algorithm with predicted cost values from HOF planning network.
     \item This paper evaluates the performance of HOF planning network in simulation and verifies the network with a physical robot system.
     
\end{itemize}

\section{Network}
\jinwook{DO}

The advantage of suggested network

\begin{itemize}
    \item We suggest a network architecture to estimates cost values of samples in the configuration space, and we can use the cost values of samples for fast path planning in the configuration space.
    \item The network structure has three layers; Cmap network, HOF network and Decoder network.
    \item The first network constructs occupancy of collision region in C-space, and it is an efficient way compared to generating cost values in C-space directly. Since cost-value depends on a goal configuration and environment, the method generating cost value directly requires update whenever the goal configuration is changed. However, our Cmap network doesn't need update if the environment is not changed.   
    \item HOF network is a neural network encodes the information of Cmap, which was generated from Cmap network, into the weights and biases of the secondary decoder network.
    \item The decoder network is a "prediction" network which estimates cost values of given sample configurations.
    \item Since the decoder network has only 256 parameters and we use only the decoder network for cost estimation for planning in a given environment, it is appropriate for fast planning. In addition, since when the environment is changed, the Cmap network and HOF network quickly update the weights and biases of decoder network, it can update network without heavy computation.
    \item Since the inference of network is very fast, we can use this network for fast path planning avoiding obstacles. 
    
\end{itemize}

\subsection{Cmap Network}

\begin{figure}
\centering
\includegraphics[width=0.9\textwidth]{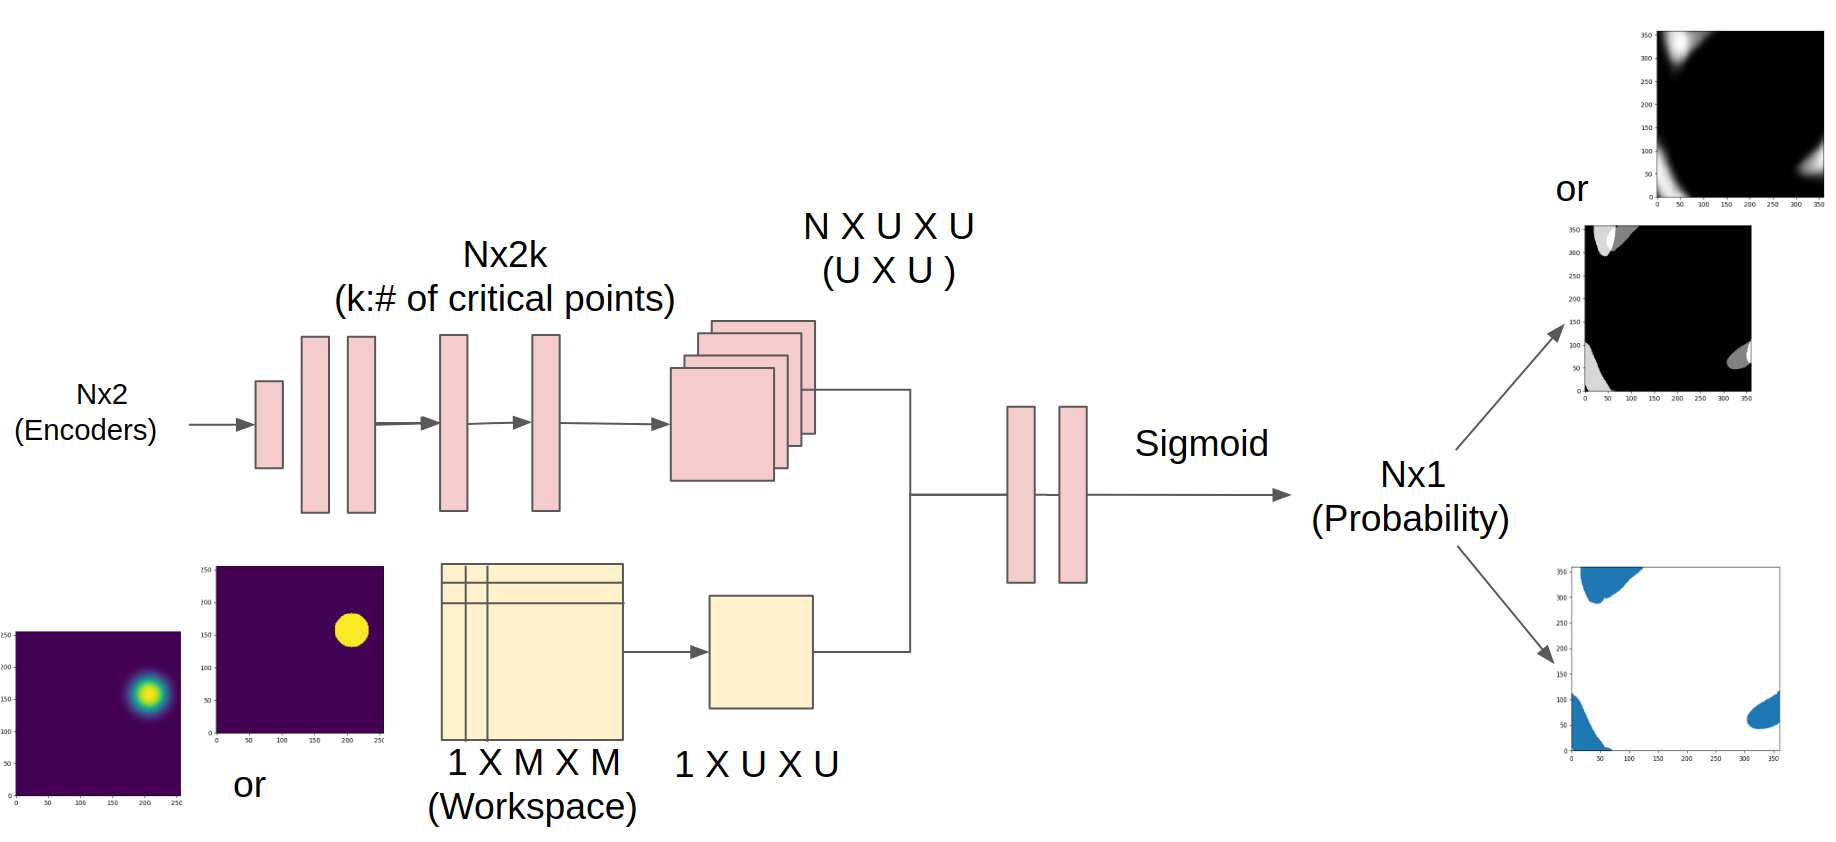}
\caption{Cmap network}
\label{cmap_net}
\end{figure}

Fig. \ref{cmap_net} shows the Configuration map (Cmap) network structure for generating collision map in the configuration space. Input of the network is workspace information (binary or continuous data with Gaussian mask) and sample configuration points for estimating collision. If we input uniform samples in configuration space, we can obtain Cmap as shown in the output of Fig. \ref{cmap_net}. We train the network with data obtained by forward kinematics of random sample configurations. Using forward kinematics, we can obtain the arm configuration (shape) in the workspace, and the network is trained to minimize the error between estimation of arm configuration and arm configuration based upon forward kinematics. Since the network can infer a lot of given sample configurations instantly, the network can generate Cmap instantly. In addition, this network can estimate the probability of collision, it is very useful for estimation of cost compared to traditional binary collision check based on forward kinematics.

Summary:

\begin{itemize}
    \item Cmap network estimates collision of given samples
    \item We train Cmap network with data obtained by forward kinematics of random sample configurations. We know the arm shape in the workspace by forward kinematics and the network learns to minimize error between the error between estimation of arm configuration and arm configuration based upon forward kinematics.
    \item The network has an advantage to estimate collision probability of sample configurations instantly; thus it generates Cmap of configuration spcae instantly.
    \item Since Cmap represents the collision C-space, it is also applicable to other planning approaches such as A* and RRTs.
    
\end{itemize}

% \begin{figure}
% \centering
% \begin{subfigure}[b]{0.42\textwidth}
% \includegraphics[width=\textwidth]{robot_concept}
% \end{subfigure}
% \begin{subfigure}[b]{0.54\textwidth}
% \includegraphics[width=\textwidth]{first_page7}  %canonical_obstacles
% \end{subfigure}
% \caption{A manipulator moves to the shelf to grasp an object. Ellipsoids mean the 90\% confidence level of the collision. The blue and magenta lines depict trees, and the black line is the final path. The red dots are collision exemplars for the GMM. (Best viewed in color)}
% \label{cck_concepts}
% \end{figure}

\subsection{Encoder Network}

\begin{figure}[t]
\centering
\subfigure[2D network]{\label{fig:2Dnet}\includegraphics[width=\textwidth]{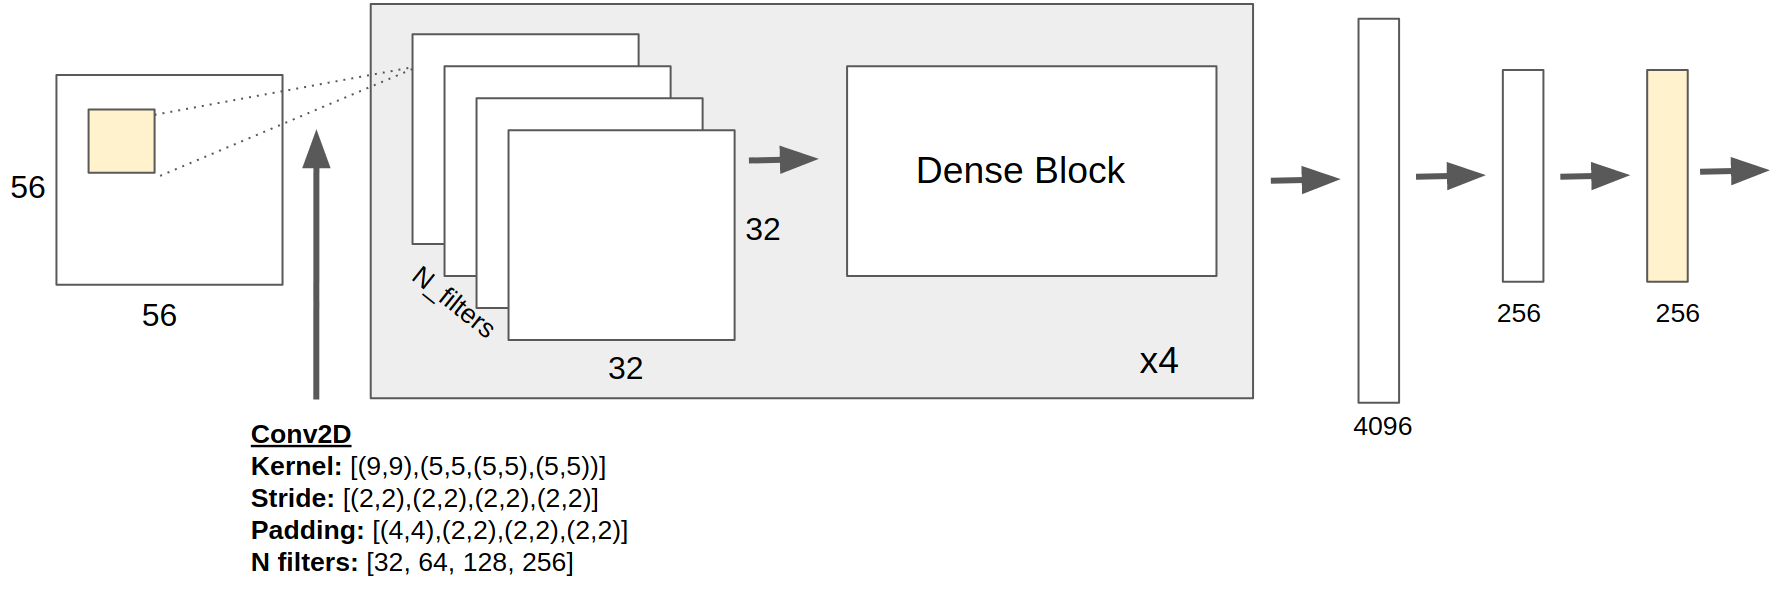}}
\hspace{5mm}
\subfigure[3D network]{\label{fig:3Dnet}\includegraphics[width=\textwidth]{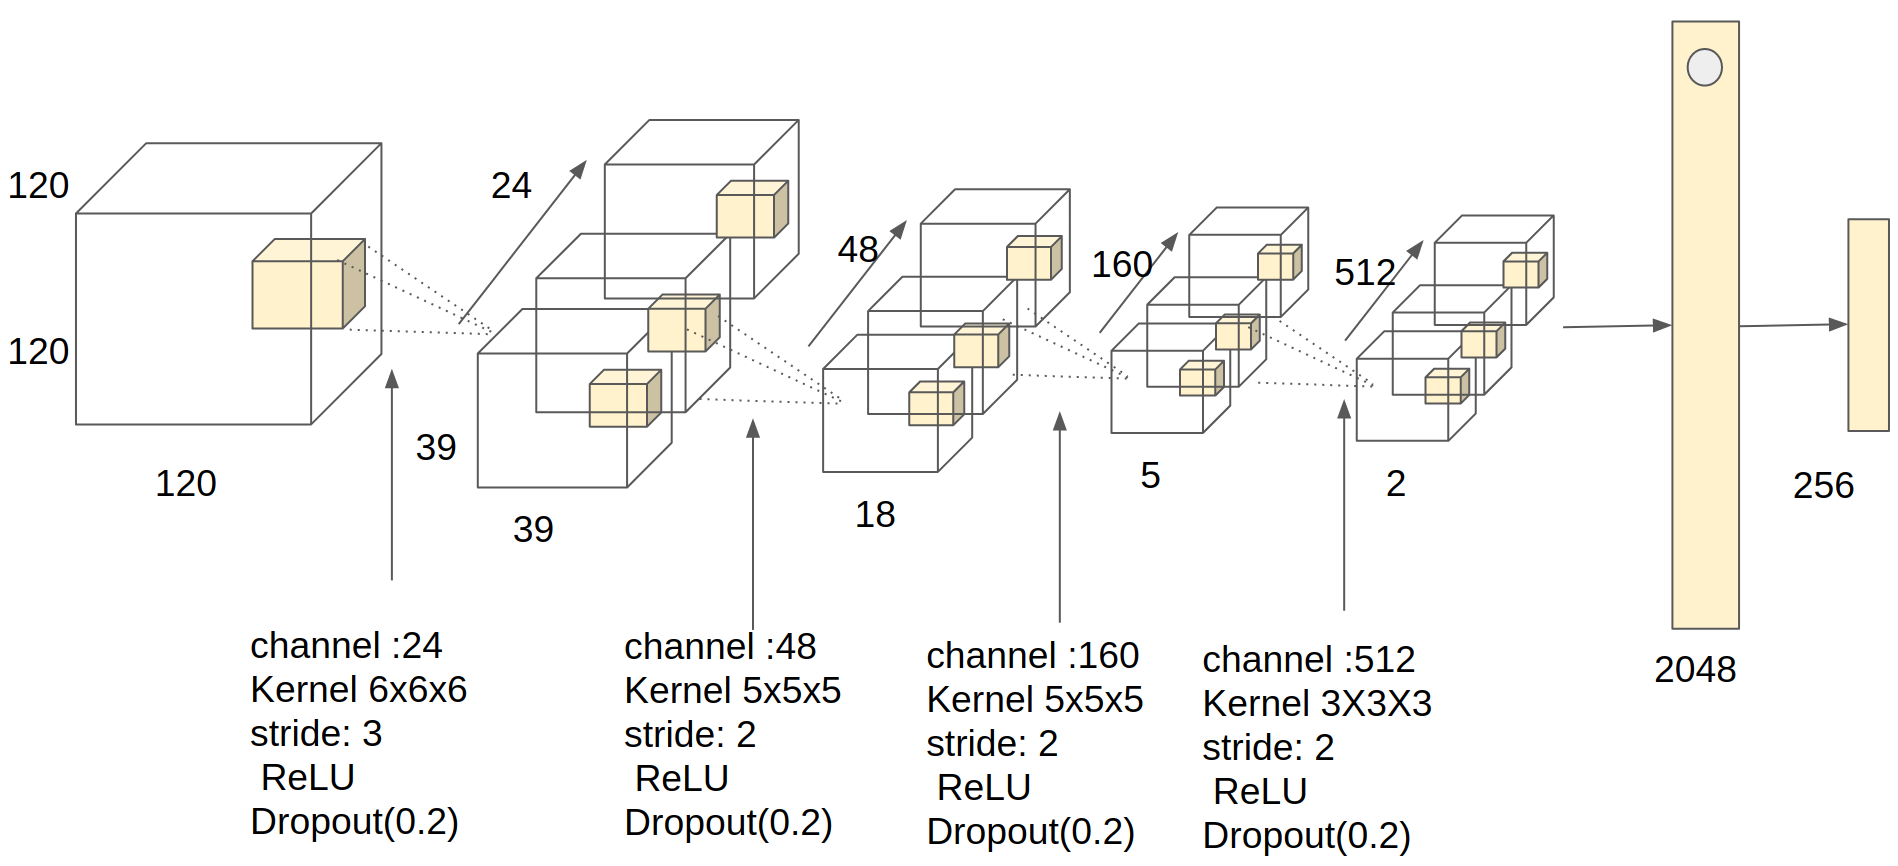}
\label{fig:networks}}
\caption{Encoder networks}
\end{figure}

% \begin{figure}[h!]
% \centering
% \includegraphics[width=\textwidth]{2d_network.png}
% \caption{2D network}
% \label{fig:2Dnet}
% \end{figure}

% \begin{figure}[h!]
% \centering
% \includegraphics[width=\textwidth]{3d_network.png}
% \caption{3D network}
% \label{fig:3Dnet}
% \end{figure}

Fig. \ref{fig:2Dnet} shows the 2D network for 2D link manipulator. The input of the encoder network is Cmap and the out of the encoder network is weights and biases of decoder network. 2D encoder is constructed by 2D convolutional neural network as shown in Fig. \ref{fig:2Dnet}. Fig. \ref{fig:3Dnet} shows the 3D network for 3D manipulator.

\subsection{Decoder}
\begin{figure}[h!]
\centering
\includegraphics[width=\textwidth]{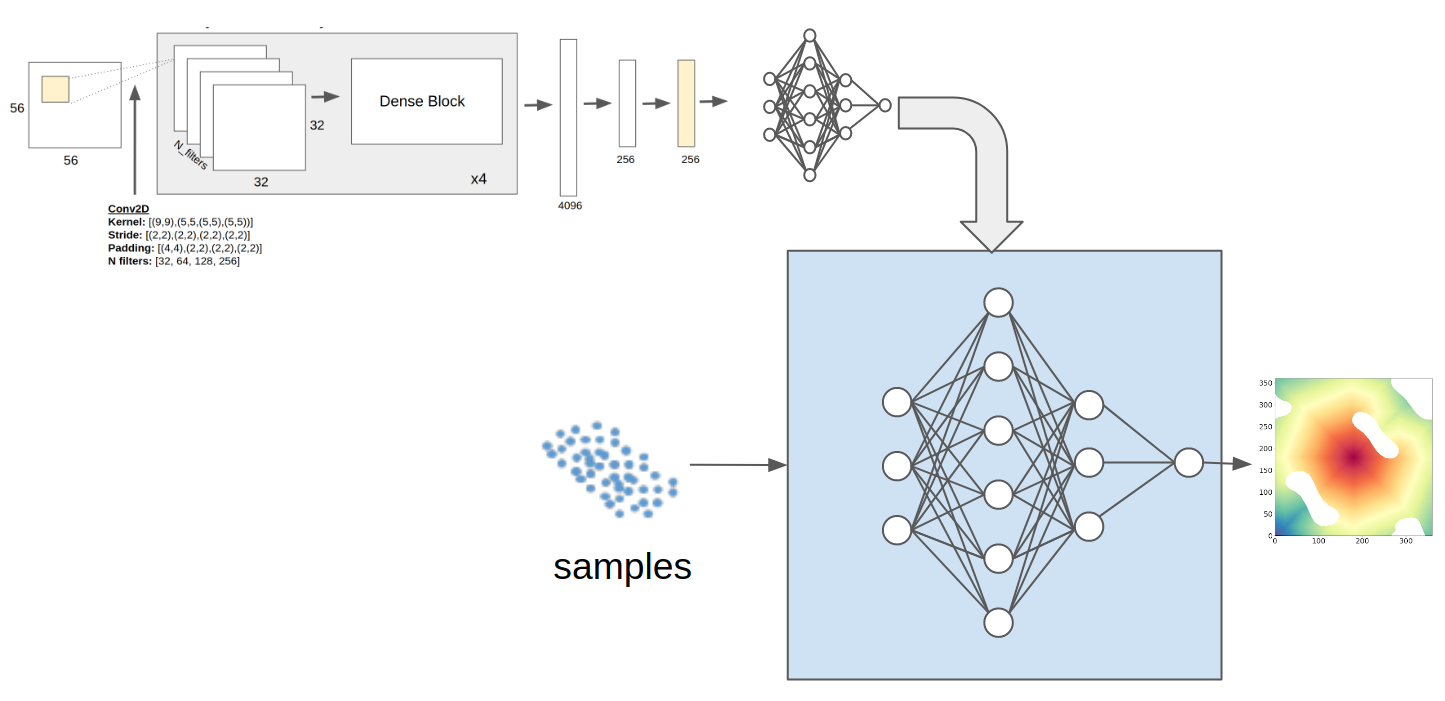}
\caption{3D network}
\label{fig:decoder}
\end{figure}
The decoder network is a "prediction" network which estimates cost values of sample configurations. 
The prediction network has 256 parameters for weights and biases which are output of encoder. The decoder constructs the network with weights to estimate a cost value of configuration points.(explain how to construct the network more detail)

\jinwook{DO}
\begin{figure}[h!]
\centering
\includegraphics[width=\textwidth]{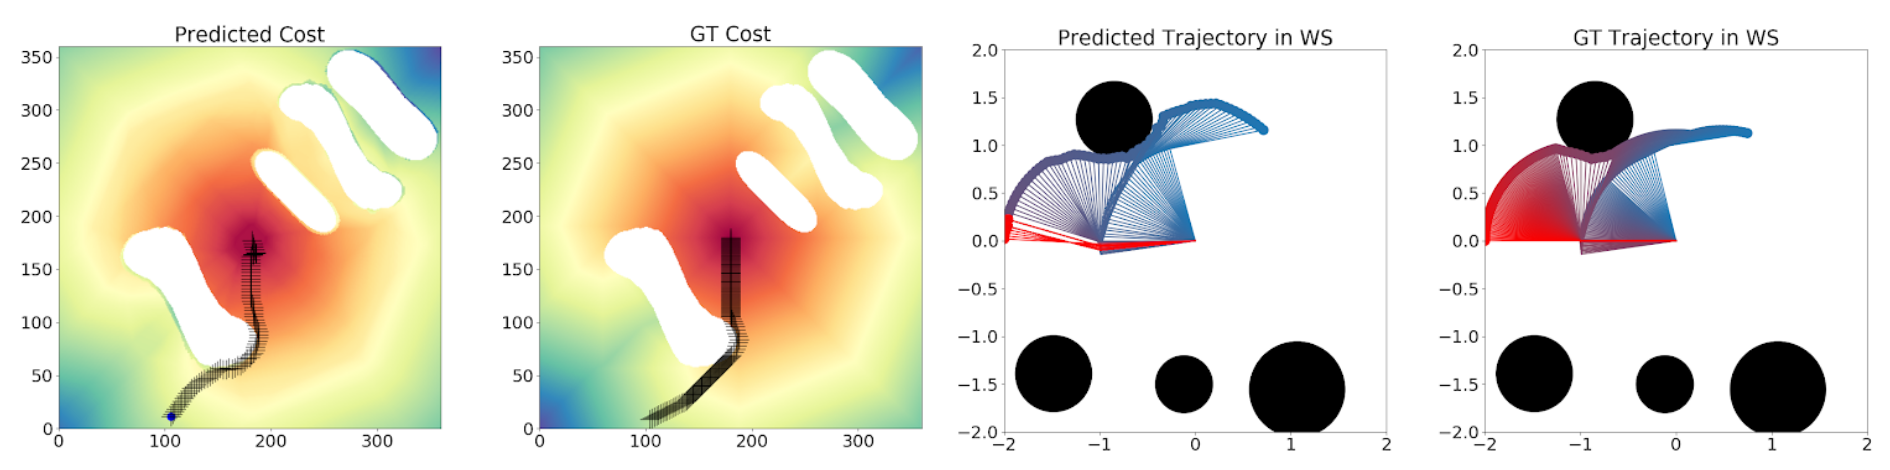}
\caption{comparison of planning results based on estimated cost and ground truth of Dijkstra}
\label{fig:planning}
\end{figure}

\begin{figure}[t]
\centering
\subfigure{\label{grd_fig:polyhedron1}\includegraphics[width=0.45\textwidth]{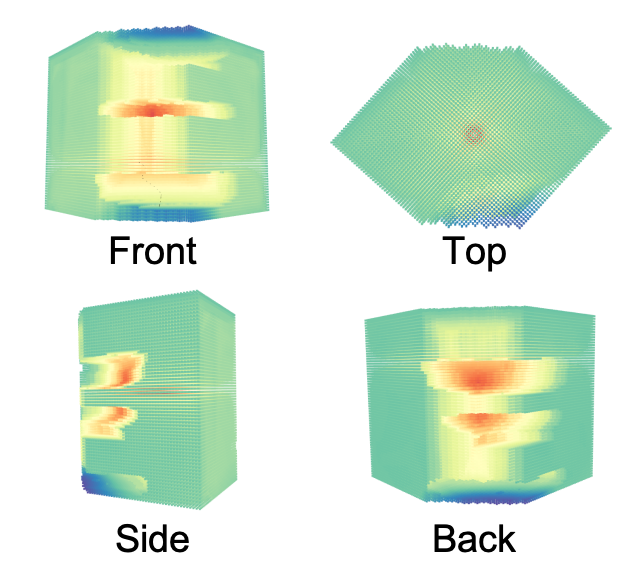} \label{}}
\hspace{5mm}
\subfigure{\includegraphics[width=0.45\textwidth]{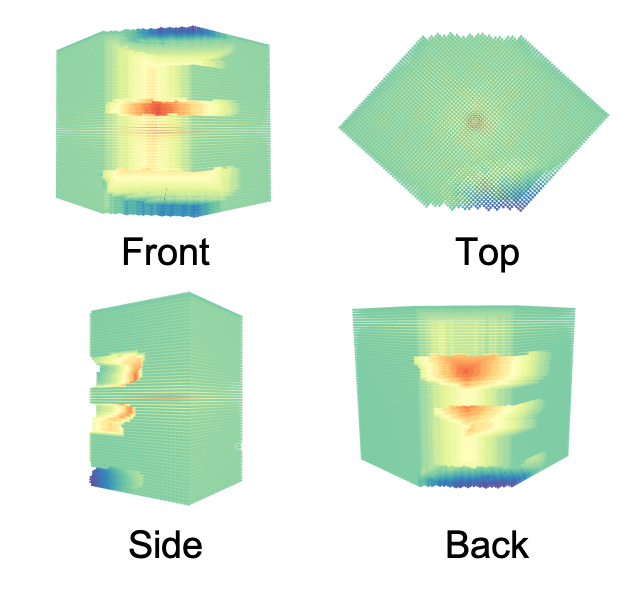}
\label{grd_fig_concept}}
\vspace{-2mm}
\caption{(left) predicted cost (right) Ground truth cost}
\label{grd_fig:polytope}
\end{figure}

\begin{figure}[t]
\centering
\subfigure{\label{grd_fig:polyhedron1}\includegraphics[width=0.45\textwidth]{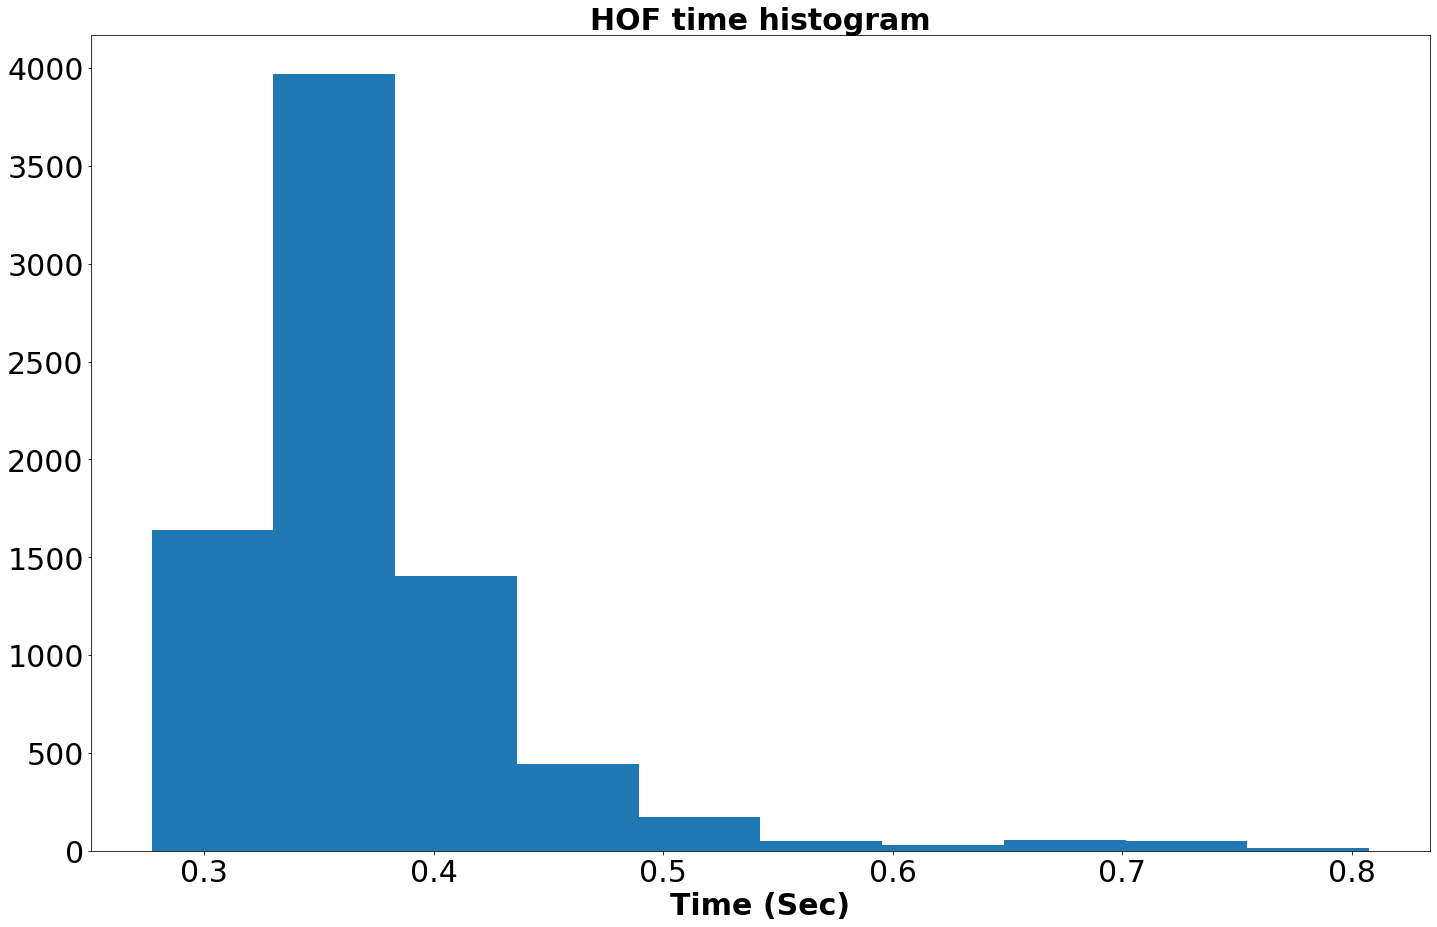} \label{}}
\hspace{5mm}
\subfigure{\includegraphics[width=0.45\textwidth]{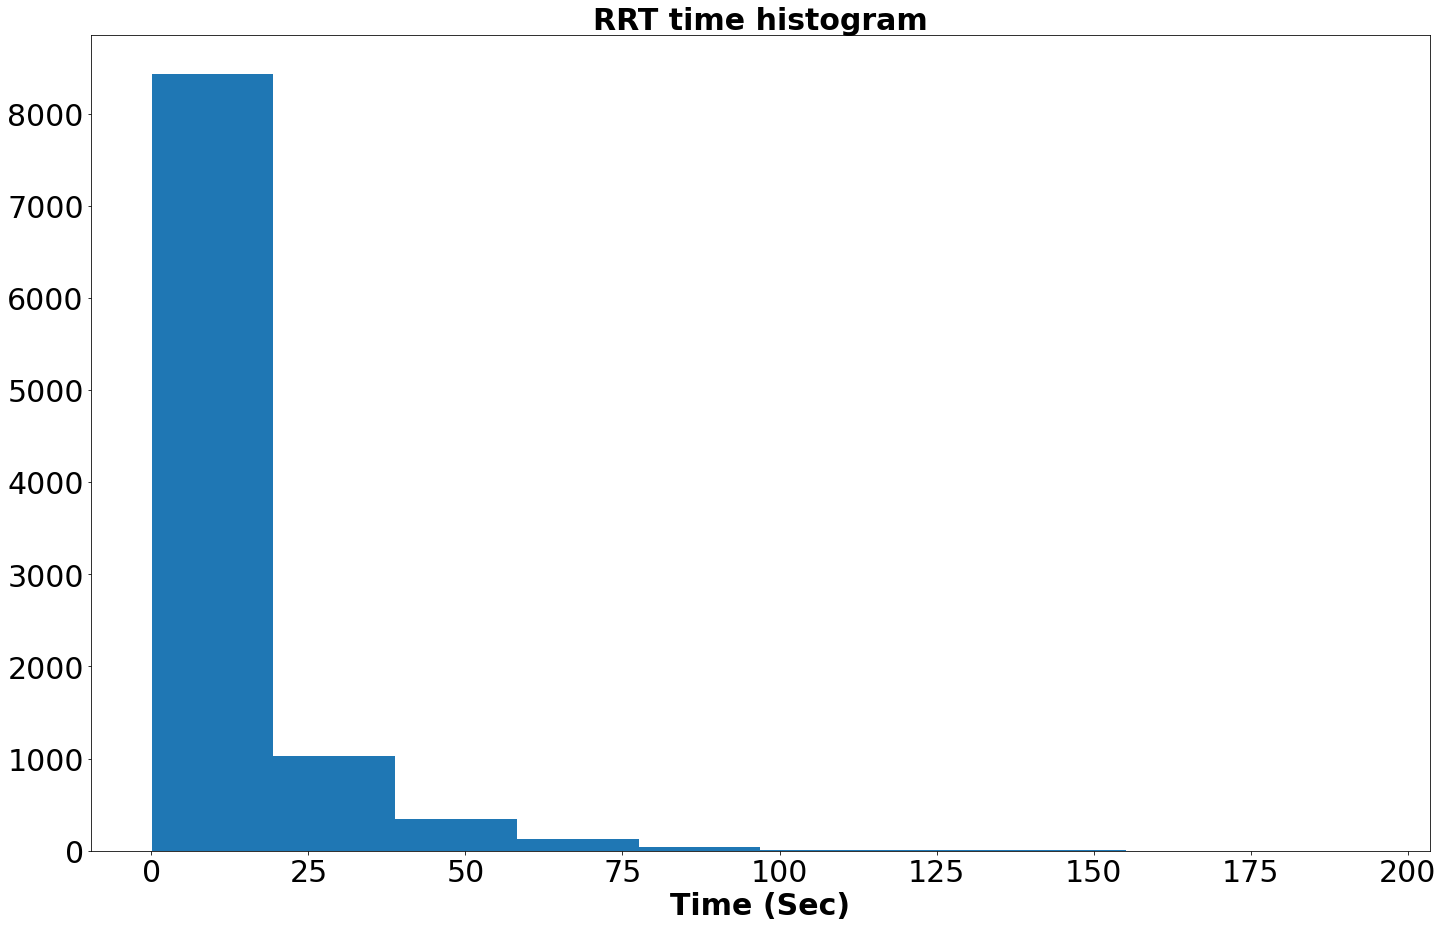}
\label{grd_fig_concept}}
\vspace{-2mm}
\caption{(left) Histogram of HOF planning time (right) Histogram of RRT planning time}
\label{grd_fig:polytope}
\end{figure}

\section{Online Path Planning}

\begin{itemize}
    \item Need a trajectory generation with the network for cost value estimation
    \item We need to find gradient of cost value and trajectory is generated to minimize the cost value following gradient (gradient descent)
    \item Since we don't have gradient function, we apply a sampling method to find a minimum gradient in a given configuration.
    \item We generate a trajectory following with a step size according to the gradient until it arrives at goal configuration.
    \item The trajectory occasionally falls into local minima; thus it gives the attractive force of the goal when it stuck in local minima. 
    \item In order to avoid collision strongly, we add a penalty cost on the boundary of collision to the output of network.
\end{itemize}

% ``I always thought something was fundamentally wrong with the universe'' \citep{adams1995hitchhiker}

% \volkan{this reads more like an opening hook ;-)}

\section{Experiments}
\jinwook{experiment list}
\begin{itemize}
    \item computation time : mean/variance (box plot) compared to RRT and Dijkstra
    \item Success rate
    \item graph : computation time w.r.t  the number of obstacles in workspace comapred to RRT and Dijkstra
    \item Optimality (Ratio of Path Lengths) compared to RRT and Dijkstra
    \item Accuracy of cost value (example trajectories)
    \item Visualization of Trajectory of end-effector in workspace (RRT and Dijkstra have jerky motion)
    \item Time allocation for cmap/hof network/planning
    \item Computational time compared with RRT* algorithm  w.r.t optimality
\end{itemize}

\subsection{Implementation Details}
\jinwook{what numbers? / what cases?}
\jinwook{what advantages?? simulation with images and test in real robot, trajectories in simulation is realistic in real robot}
\begin{itemize}
    \item We can train the network with workspace images and it can generate trajectories of real robot. 
\end{itemize}

\subsubsection{Data Collection}
\jinwook{Galen, could you finish filling this section?}
In all our experiments, we learn the network  by using the cost generated based on Dijkstra. For Dijkstra we select the grid size to represent the cost value sufficiently in C-space.
We select ?? degrees for the grid size in Dijkstra for 2DoF manipulator.
For the data size~~~ 
\begin{itemize}
    \item How to Generate data (20K training examples)
    \item explain shortly Dijkstra why we choose it and how to discretize
\end{itemize}
\subsubsection{Learning of network}
\jinwook{DO}
\begin{itemize}
    \item adaptive sampling along the border of the collision regions based on the probability of collision or laplacian method of cmap
    \item \jinwook{what do we have methods for better training??}
\end{itemize}

\subsection{Simulation}

\begin{itemize}
    \item Training curves for datasets built with various sigma values for gaussian blurring (0, 5, 10) \volkan{these need to be tied to questions around the method. Do we think that this is an important parameter or is this for initial investigation?}
    \item How does gaussian blurring of the input workspace image affect the performance of the network? Do we achieve faster convergence during training time? Do we see performance increases? How does it affect generalization?

\jinwook{Galen, the number of epoch is too small. Also could you give the data to me? I will draw again.}
    \item How does the success rate of trajectories change as we increase the number of obstacles 
    \item Success rate as we increase the number of obstacles in the workspace. We can also play around with the size of the obstacles. (I'm actually curious how this would turn out because different workspaces for 2dof doesn't change the shapes of the configuration space THAT much) \volkan{performance as we increase the number and complexity of the obstacles. Explain how you measure complexity -- is it size distribution, aspect ratio etc.}
    \item Comparison of runtimes for 2dof and 3dof compared to RRT* and A*
    \jinwook{How to compare it with A*? Do you think A* is in C-space or workspace? Maybe C-space. In that case, it requires discretization. so it is a weakness of A* -> Conclusion : A* uses the Cmap results}
    \item Comparison of trajectory lengths between our method and RRT* and A*
    \item 2dof and 3dof example trajectories (where it ISNT moving to the center of the configuration space. (aka need to code up this transformation)
    \item \jinwook{Please include comparison of cost value following  trajectories between 100 random start and goal points}
\end{itemize}

\begin{figure}[h!]
\centering
\includegraphics[width=\textwidth]{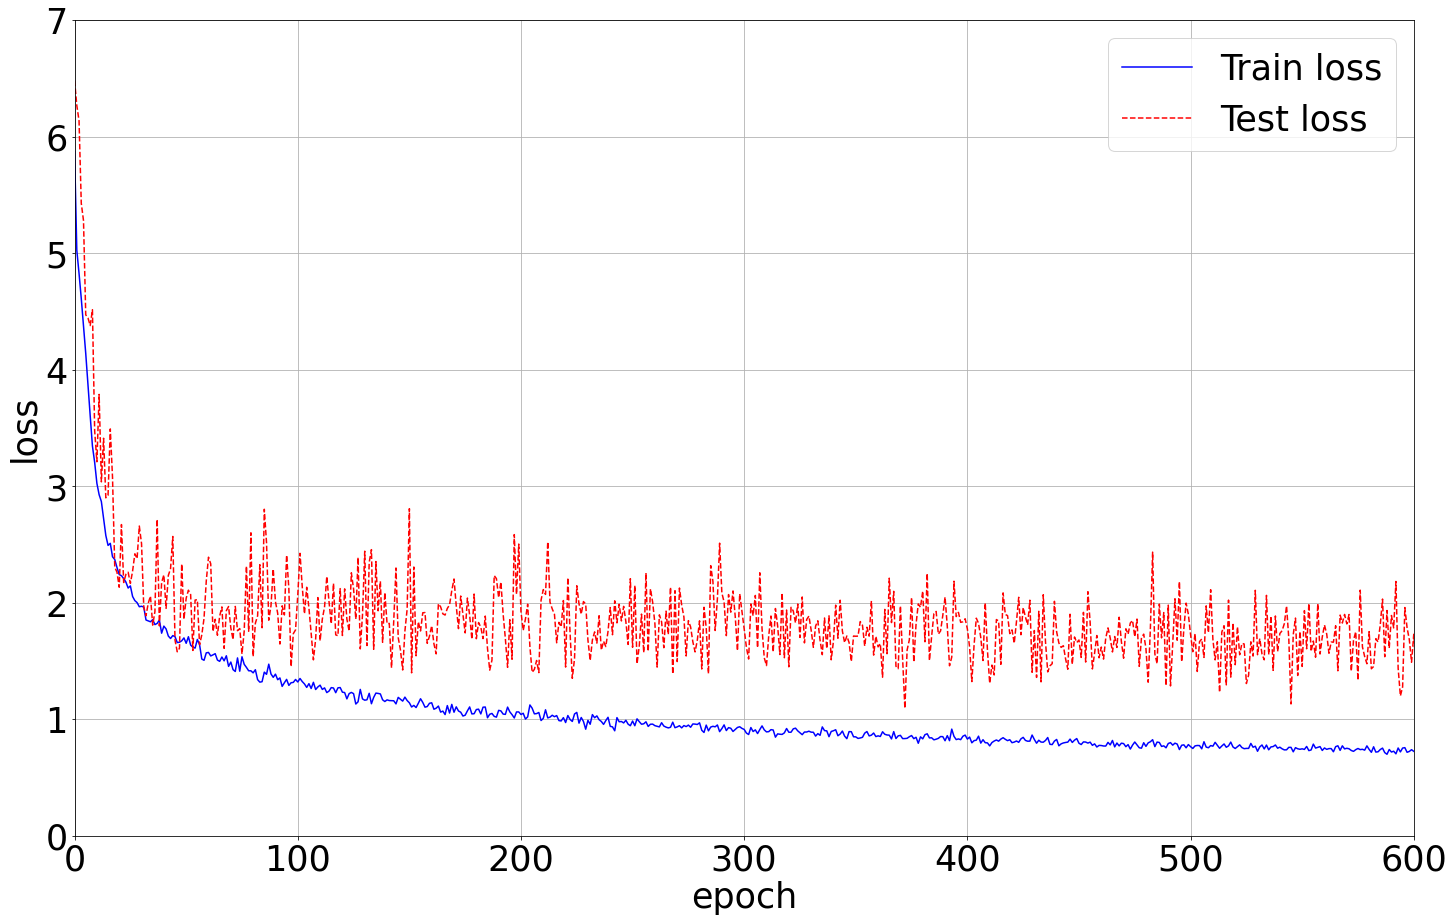}
\caption{Learning curve for 3D network}
\label{fig:learning_curve}
\end{figure}

\subsection{Physical Robot Experiments}

\begin{figure}[t]
\centering
\subfigure{\label{grd_fig:polyhedron1}\includegraphics[width=0.45\textwidth]{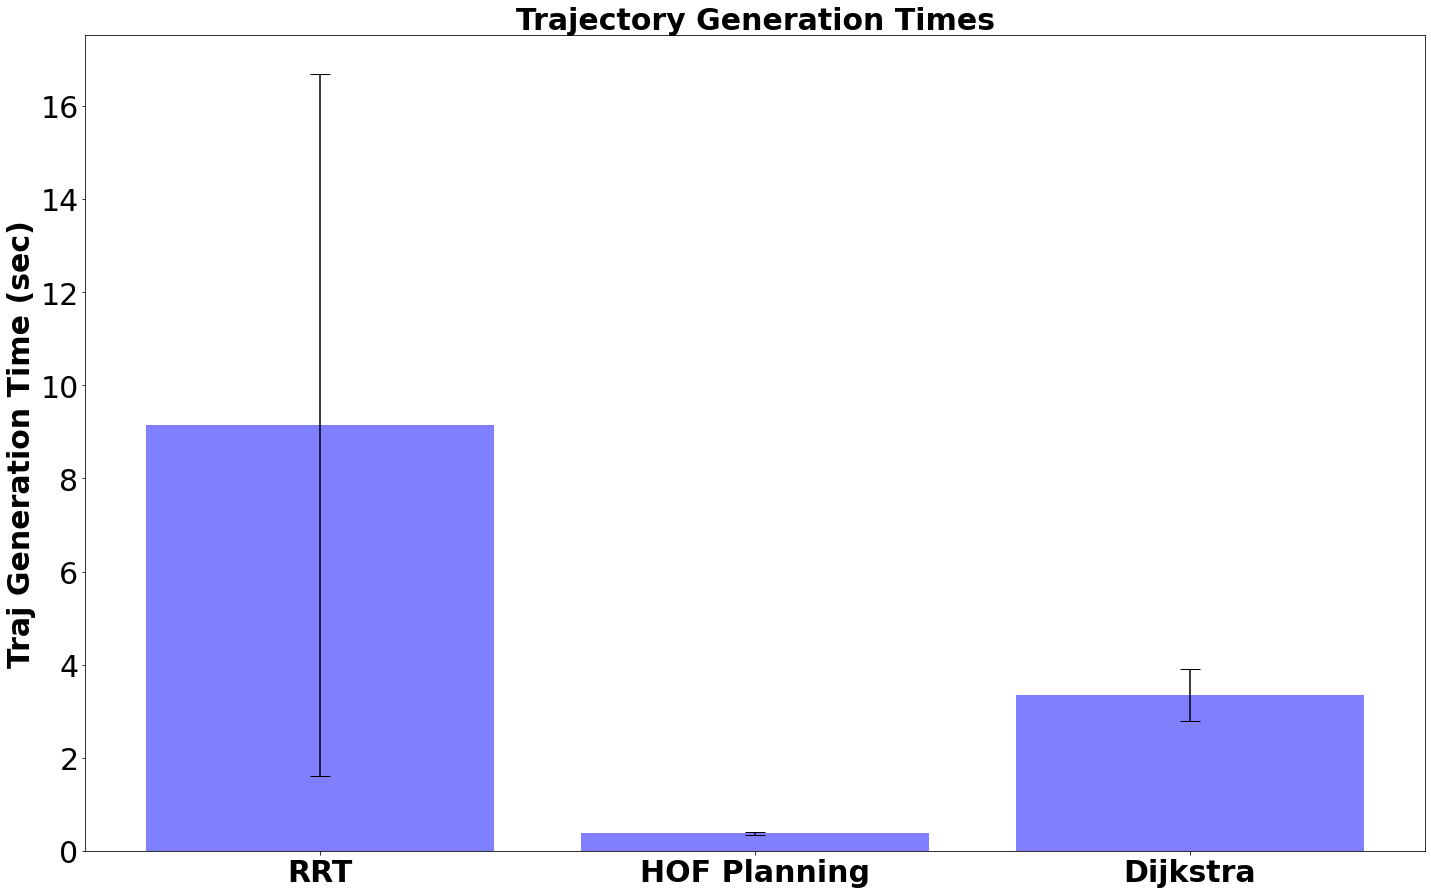} \label{grd_fig_polyhedron}}
\hspace{5mm}
\subfigure{\includegraphics[width=0.45\textwidth]{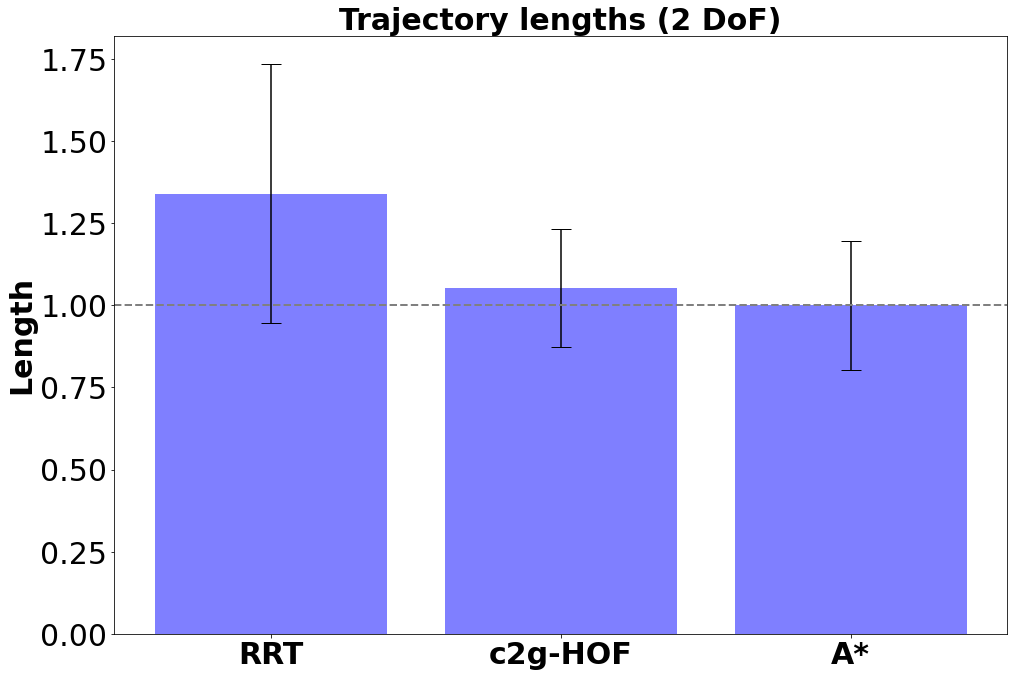}
\label{grd_fig_concept}}
\vspace{-2mm}
\caption{(left) Planning time (right) Trajectory length}
\label{grd_fig:polytope}
\end{figure}

\jinwook{book shelf is good example for 2.5D workspace}
\begin{itemize}
    \item 2-DoF and 3-DoF experiments with circular pieces of paper. At the very least, this would be a sanity check for us to make sure that we can execute trajectories on the robot
    \item 2-DoF and 3-DoF experiments with more complicated environments. I was thinking: local minima in the workspace as well as local minima in the configuration space
    \item Marquee experiment: have the 3-DoF robot move around obstacle and into a tight space
    
\end{itemize}

\section{Conclusion}

qqq
